# Supplementary material for: A Lost Opportunity for Vision-Language Models: A Comparative Study of Online Test-Time Adaptation for Vision-Language Models
Source: arXiv:2405.14977 source file (2024-09-09)
Supplement: Supplementary file 1 [file supplementaries.tex]

\begin{table*}[t]

\centering
\caption{Online classification error rate~(\%) for CLIP with a RN50 backbone pretrained by OpenAI. The model comprises 102.01 million parameters and requires 18.18 billion FLOPS.}
\vskip -0.1in
\scalebox{0.75}{
\tabcolsep4pt
\begin{tabular}{l|l|ccccccccccccccccc|c}\hline
    Method & Prompt & \rotatebox[origin=c]{70}{ImageNet} & \rotatebox[origin=c]{70}{ImageNet-C} & \rotatebox[origin=c]{70}{ImageNet-A} & \rotatebox[origin=c]{70}{ImageNet-V2} & \rotatebox[origin=c]{70}{ImageNet-R} & \rotatebox[origin=c]{70}{ImageNet-S} & \rotatebox[origin=c]{70}{ImageNet-D109} & \rotatebox[origin=c]{70}{Flower102} & \rotatebox[origin=c]{70}{DTD} & \rotatebox[origin=c]{70}{Pets} & \rotatebox[origin=c]{70}{Cars} & \rotatebox[origin=c]{70}{UCF101} & \rotatebox[origin=c]{70}{Caltech101} & \rotatebox[origin=c]{70}{Food101} & \rotatebox[origin=c]{70}{SUN397} & \rotatebox[origin=c]{70}{Aircraft} & \rotatebox[origin=c]{70}{EuroSAT} & Avg. \\
    \hline
Source & Single & 41.8 & 89.0 & 78.3 & 48.5 & 44.1 & 66.7 & 41.2 & 39.0 & 60.1 & 16.4 & 44.4 & 41.7 & 14.1 & 26.2 & 41.4 & 84.4 & 75.8 & 50.2 \\ 
Source & Ensemble & 40.2 & 88.3 & 77.3 & 47.2 & 39.4 & 64.6 & 38.7 & 38.7 & 58.3 & 16.7 & 44.0 & 40.6 & 13.8 & 24.3 & 39.8 & 83.0 & 61.8 & 48.0 \\ 
Source & CuPL & 38.5 & 87.7 & 76.2 & 45.4 & 40.0 & 64.3 & 38.6 & - & - & - & - & - & - & - & - & - & - & -\ \\ 
Source & All Prompts & 38.7 & 87.8 & 76.2 & 45.9 & 38.9 & 63.7 & 38.2 & - & - & - & - & - & - & - & - & - & - & -\ \\ 
\hline
TPT & a photo of a & 39.2 & 88.6 & 73.7 & 45.5 & 41.1 & 64.8 & 38.4 & 37.8 & 59.0 & 15.2 & 41.4 & 40.3 & 13.1 & 25.1 & 38.7 & 82.8 & 72.0 & 48.0 \\ 
VTE & Ensemble & 38.6 & 88.5 & 66.5 & 44.5 & 37.8 & 63.0 & 36.1 & 41.6 & 59.4 & 17.3 & 41.3 & 41.0 & 13.5 & 26.4 & 39.1 & 81.1 & 72.7 & 47.5 \\ 
\hline
TENT & Ensemble & 53.3 & 97.8 & 89.8 & 59.8 & 56.6 & 82.1 & 50.7 & 88.6 & 78.2 & 52.0 & 91.3 & 61.2 & 35.9 & 90.2 & 60.1 & 95.8 & 87.8 & 72.4 \\ 
ETA & Ensemble & 50.2 & 99.8 & 89.5 & 58.8 & 53.4 & 78.9 & 49.5 & 88.6 & 78.3 & 52.2 & 91.0 & 61.5 & 36.3 & 85.2 & 58.4 & 95.8 & 86.9 & 71.4 \\ 
SAR & Ensemble & 53.7 & 96.2 & 89.8 & 59.9 & 57.4 & 81.8 & 51.0 & 88.4 & 78.2 & 52.0 & 91.0 & 61.1 & 36.5 & 88.1 & 60.2 & 95.7 & 86.9 & 72.2 \\ 
DeYO & Ensemble & 50.1 & 99.8 & 89.4 & 58.3 & 52.6 & 79.9 & 48.2 & 88.9 & 77.9 & 51.2 & 90.7 & 60.5 & 34.7 & 89.5 & 57.8 & 96.3 & 89.1 & 71.5 \\ 
CMF & Ensemble & 48.0 & 93.3 & 88.4 & 57.2 & 47.0 & 75.2 & 44.6 & 88.8 & 78.2 & 44.6 & 90.2 & 57.0 & 33.5 & 80.1 & 54.1 & 95.7 & 91.1 & 68.6 \\ 
ROID & Ensemble & 50.2 & 91.7 & 89.0 & 57.2 & 50.2 & 77.8 & 47.1 & 89.0 & 77.9 & 44.8 & 90.4 & 57.4 & 33.1 & 83.9 & 55.9 & 95.9 & 90.6 & 69.5 \\
    \hline
\end{tabular}}
\label{tab:detailed_rn50}
\end{table*}
\begin{table*}[t]

\centering
\caption{Online classification error rate~(\%) for CLIP with a ViT-B-16 backbone pretrained by OpenAI. The model comprises 149.62 million parameters and requires 41.09 billion FLOPS.}
\vskip -0.1in
\scalebox{0.75}{
\tabcolsep4pt
\begin{tabular}{l|l|ccccccccccccccccc|c}\hline
    Method & Prompt & \rotatebox[origin=c]{70}{ImageNet} & \rotatebox[origin=c]{70}{ImageNet-C} & \rotatebox[origin=c]{70}{ImageNet-A} & \rotatebox[origin=c]{70}{ImageNet-V2} & \rotatebox[origin=c]{70}{ImageNet-R} & \rotatebox[origin=c]{70}{ImageNet-S} & \rotatebox[origin=c]{70}{ImageNet-D109} & \rotatebox[origin=c]{70}{Flower102} & \rotatebox[origin=c]{70}{DTD} & \rotatebox[origin=c]{70}{Pets} & \rotatebox[origin=c]{70}{Cars} & \rotatebox[origin=c]{70}{UCF101} & \rotatebox[origin=c]{70}{Caltech101} & \rotatebox[origin=c]{70}{Food101} & \rotatebox[origin=c]{70}{SUN397} & \rotatebox[origin=c]{70}{Aircraft} & \rotatebox[origin=c]{70}{EuroSAT} & Avg. \\
    \hline
Source & Single & 33.3 & 75.5 & 52.3 & 39.2 & 26.0 & 53.9 & 29.5 & 32.6 & 55.4 & 11.8 & 34.8 & 34.9 & 7.1 & 16.2 & 37.4 & 76.2 & 58.5 & 39.7\\ 
Source & Ensemble & 31.7 & 73.8 & 49.9 & 38.1 & 22.5 & 51.7 & 27.5 & 34.2 & 54.6 & 11.8 & 33.6 & 32.6 & 7.0 & 15.5 & 34.6 & 76.5 & 51.8 & 38.1\\ 
Source & CuPL & 30.4 & 73.3 & 49.3 & 36.7 & 22.9 & 51.0 & 28.0 & - & - & - & - & - & - & - & - & - & - & -\\ 
Source & All Prompts & 30.3 & 73.0 & 49.0 & 36.9 & 22.0 & 50.6 & 27.2 & - & - & - & - & - & - & - & - & - & - & -\\ 
\hline
TPT & a photo of a & 31.0 & 75.1 & 45.7 & 36.5 & 23.0 & 52.2 & 26.8 & 30.9 & 52.7 & 12.8 & 34.0 & 32.5 & 6.3 & 15.2 & 34.6 & 76.7 & 57.2 & 37.8\\ 
VTE & Ensemble & 29.6 & 74.4 & 37.3 & 34.9 & 19.6 & 49.8 & 24.6 & 34.5 & 52.7 & 13.0 & 31.0 & 33.0 & 6.7 & 16.6 & 33.5 & 75.9 & 52.4 & 36.4\\ 
\hline
TENT & Ensemble & 31.6 & 75.4 & 49.6 & 38.1 & 21.6 & 51.6 & 27.2 & 34.2 & 54.3 & 11.6 & 33.6 & 32.3 & 6.9 & 15.8 & 34.4 & 76.5 & 43.3 & 37.5\\ 
ETA & Ensemble & 32.1 & 69.1 & 49.3 & 38.3 & 21.7 & 50.9 & 26.9 & 34.0 & 54.4 & 11.3 & 33.5 & 32.1 & 7.0 & 16.0 & 33.9 & 76.2 & 50.7 & 37.5\\ 
SAR & Ensemble & 32.0 & 70.0 & 49.2 & 38.3 & 21.8 & 51.5 & 27.0 & 33.9 & 54.4 & 11.5 & 34.1 & 32.5 & 7.0 & 15.7 & 34.8 & 76.4 & 44.7 & 37.3\\ 
DeYO & Ensemble & 32.4 & 71.3 & 48.9 & 38.4 & 21.7 & 51.5 & 27.0 & 34.2 & 54.3 & 11.3 & 34.1 & 32.1 & 7.2 & 16.0 & 35.0 & 76.2 & 50.1 & 37.7\\ 
CMF & Ensemble & 31.9 & 66.1 & 49.6 & 38.3 & 20.9 & 50.4 & 25.7 & 33.8 & 54.4 & 11.5 & 33.8 & 32.0 & 6.9 & 15.7 & 33.6 & 76.3 & 36.5 & 36.3\\ 
ROID & Ensemble & 31.7 & 65.7 & 49.3 & 38.2 & 21.1 & 50.9 & 26.3 & 33.6 & 54.2 & 11.4 & 33.4 & 31.9 & 6.9 & 15.8 & 33.4 & 76.1 & 36.3 & 36.2 \\
    \hline
\end{tabular}}
\label{tab:detailed_vit_b_16}
\end{table*}

\begin{table*}[t]

\centering
\caption{Online classification error rate~(\%) for CLIP with a EVA02-B-16 backbone. The model comprises 149.69 million parameters and requires 41.09 billion FLOPS.}
\vskip -0.1in
\scalebox{0.75}{
\tabcolsep4pt
\begin{tabular}{l|l|ccccccccccccccccc|c}\hline
    Method & Prompt & \rotatebox[origin=c]{70}{ImageNet} & \rotatebox[origin=c]{70}{ImageNet-C} & \rotatebox[origin=c]{70}{ImageNet-A} & \rotatebox[origin=c]{70}{ImageNet-V2} & \rotatebox[origin=c]{70}{ImageNet-R} & \rotatebox[origin=c]{70}{ImageNet-S} & \rotatebox[origin=c]{70}{ImageNet-D109} & \rotatebox[origin=c]{70}{Flower102} & \rotatebox[origin=c]{70}{DTD} & \rotatebox[origin=c]{70}{Pets} & \rotatebox[origin=c]{70}{Cars} & \rotatebox[origin=c]{70}{UCF101} & \rotatebox[origin=c]{70}{Caltech101} & \rotatebox[origin=c]{70}{Food101} & \rotatebox[origin=c]{70}{SUN397} & \rotatebox[origin=c]{70}{Aircraft} & \rotatebox[origin=c]{70}{EuroSAT} & Avg. \\
    \hline
Source & Single & 25.5 & 64.5 & 46.5 & 33.3 & 18.9 & 42.9 & 26.1 & 24.5 & 50.1 & 10.0 & 20.9 & 31.7 & 2.8 & 15.6 & 29.1 & 77.3 & 45.1 & 33.2\\
Source & Ensemble & 25.3 & 63.8 & 46.1 & 33.0 & 17.6 & 42.3 & 25.0 & 25.1 & 47.7 & 10.2 & 20.9 & 31.2 & 3.6 & 15.1 & 29.1 & 76.7 & 37.8 & 32.4\\
Source & CuPL & 24.8 & 63.9 & 45.8 & 32.5 & 19.3 & 42.7 & 25.2 & - & - & - & - & - & - & - & - & - & - & -\\
Source & All Prompts & 24.6 & 63.5 & 45.4 & 32.2 & 17.5 & 42.1 & 24.8 & - & - & - & - & - & - & - & - & - & - & -\\
\hline
EnsembleCLIP & Ensemble & 23.6 & 63.2 & 27.9 & 30.6 & 14.4 & 40.7 & 21.9 & 26.6 & 46.1 & 11.3 & 19.4 & 32.0 & 3.6 & 15.9 & 30.0 & 76.4 & 48.8 & 31.3\\
\hline
TENT & Ensemble & 25.3 & 94.6 & 43.7 & 32.8 & 15.7 & 41.6 & 32.3 & 25.2 & 48.2 & 10.1 & 20.1 & 31.0 & 3.5 & 15.0 & 29.5 & 77.4 & 34.4 & 34.1\\
ETA & Ensemble & 25.7 & 55.4 & 43.6 & 32.8 & 15.3 & 41.4 & 22.9 & 25.4 & 47.8 & 10.2 & 20.3 & 30.0 & 3.8 & 14.8 & 29.5 & 77.0 & 37.8 & 31.4\\
SAR & Ensemble & 25.1 & 57.4 & 44.3 & 32.8 & 16.6 & 41.7 & 24.2 & 25.0 & 47.9 & 10.1 & 20.1 & 30.8 & 3.7 & 15.1 & 29.1 & 77.2 & 38.0 & 31.7\\
DeYO & Ensemble & 26.0 & 57.4 & 42.4 & 32.8 & 15.4 & 41.9 & 23.8 & 24.6 & 48.5 & 10.4 & 20.4 & 30.3 & 3.5 & 15.3 & 29.6 & 79.0 & 64.5 & 33.3\\
CMF & Ensemble & 25.9 & 51.5 & 43.8 & 33.1 & 15.2 & 41.8 & 22.6 & 25.9 & 49.5 & 9.3 & 21.4 & 30.1 & 4.0 & 15.0 & 29.5 & 78.7 & 44.6 & 31.9\\
ROID & Ensemble & 25.4 & 50.8 & 43.2 & 32.8 & 15.1 & 41.3 & 22.8 & 25.9 & 49.5 & 9.2 & 21.0 & 29.7 & 4.0 & 15.1 & 29.1 & 78.5 & 42.0 & 31.5\\
    \hline
\end{tabular}}
\label{tab:detailed_eva02_b_16}
\end{table*}

\begin{table*}[t]

\centering
\caption{Online classification error rate~(\%) for CLIP with a ViT-L-14 backbone pretrained by OpenAI. The model comprises 427.62 million parameters and requires 175.33 billion FLOPS.}
\vskip -0.1in
\scalebox{0.75}{
\tabcolsep4pt
\begin{tabular}{l|l|ccccccccccccccccc|c}\hline
    Method & Prompt & \rotatebox[origin=c]{70}{ImageNet} & \rotatebox[origin=c]{70}{ImageNet-C} & \rotatebox[origin=c]{70}{ImageNet-A} & \rotatebox[origin=c]{70}{ImageNet-V2} & \rotatebox[origin=c]{70}{ImageNet-R} & \rotatebox[origin=c]{70}{ImageNet-S} & \rotatebox[origin=c]{70}{ImageNet-D109} & \rotatebox[origin=c]{70}{Flower102} & \rotatebox[origin=c]{70}{DTD} & \rotatebox[origin=c]{70}{Pets} & \rotatebox[origin=c]{70}{Cars} & \rotatebox[origin=c]{70}{UCF101} & \rotatebox[origin=c]{70}{Caltech101} & \rotatebox[origin=c]{70}{Food101} & \rotatebox[origin=c]{70}{SUN397} & \rotatebox[origin=c]{70}{Aircraft} & \rotatebox[origin=c]{70}{EuroSAT} & Avg. \\
    \hline
Source & Single & 26.5 & 60.5 & 31.3 & 32.1 & 14.6 & 42.1 & 24.2 & 24.1 & 47.4 & 6.8 & 23.2 & 27.3 & 5.2 & 11.4 & 32.5 & 69.7 & 44.7 & 30.8\\ 
Source & Ensemble & 24.5 & 58.6 & 29.3 & 30.1 & 12.2 & 40.4 & 22.4 & 24.4 & 43.3 & 7.0 & 22.1 & 25.0 & 5.5 & 10.8 & 30.9 & 68.1 & 39.3 & 29.1\\ 
Source & CuPL & 23.4 & 57.7 & 28.2 & 29.2 & 12.3 & 40.0 & 22.5 & - & - & - & - & - & - & - & - & - & - & -\\ 
Source & All Prompts & 23.5 & 57.5 & 28.2 & 29.0 & 11.8 & 39.7 & 22.1 & - & - & - & - & - & - & - & - & - & - & -\\ 
\hline
TPT & a photo of a & 24.5 & 59.0 & 25.2 & 29.9 & 12.1 & 40.2 & 22.0 & 23.5 & 46.1 & 6.4 & 22.3 & 25.5 & 4.4 & 10.9 & 29.8 & 68.7 & 48.0 & 29.3\\ 
VTE & Ensemble & 23.0 & 59.5 & 20.4 & 28.4 & 10.3 & 38.9 & 20.5 & 26.2 & 41.9 & 7.1 & 21.6 & 24.6 & 4.2 & 11.7 & 29.3 & 66.1 & 46.4 & 28.2\\ 
\hline
TENT & Ensemble & 24.6 & 56.1 & 29.3 & 30.3 & 12.1 & 40.1 & 22.1 & 24.4 & 43.2 & 6.9 & 22.2 & 24.9 & 5.6 & 10.8 & 30.8 & 68.0 & 36.5 & 28.7\\ 
ETA & Ensemble & 24.6 & 53.8 & 28.9 & 30.4 & 11.9 & 39.6 & 21.7 & 24.3 & 43.1 & 7.0 & 21.7 & 24.7 & 5.6 & 10.8 & 30.5 & 67.8 & 39.3 & 28.6\\ 
SAR & Ensemble & 24.6 & 54.9 & 28.9 & 30.3 & 11.8 & 39.8 & 21.9 & 24.3 & 43.2 & 6.9 & 22.1 & 24.9 & 5.6 & 10.7 & 30.4 & 68.0 & 36.2 & 28.5\\ 
DeYO & Ensemble & 24.6 & 54.3 & 28.6 & 30.5 & 11.6 & 39.6 & 21.3 & 24.3 & 43.1 & 6.8 & 21.8 & 24.9 & 5.7 & 10.9 & 30.7 & 67.9 & 38.1 & 28.5\\ 
CMF & Ensemble & 24.2 & 50.6 & 28.2 & 30.0 & 11.1 & 38.6 & 20.4 & 24.1 & 43.0 & 6.6 & 21.9 & 24.7 & 5.6 & 10.7 & 30.1 & 67.4 & 32.2 & 27.6\\ 
ROID & Ensemble & 24.3 & 51.4 & 28.4 & 30.0 & 11.6 & 39.3 & 21.5 & 23.9 & 43.3 & 6.6 & 21.8 & 24.7 & 5.6 & 10.7 & 30.1 & 67.6 & 32.3 & 27.8\\
    \hline
\end{tabular}}
\label{tab:detailed_vit_l_14}
\end{table*}
\begin{table*}[t]

\centering
\caption{Online classification error rate~(\%) for CLIP with a EVA02-L-14 backbone. The model comprises 427.76 million parameters and requires 175.3 billion FLOPS.}
\vskip -0.1in
\scalebox{0.75}{
\tabcolsep4pt
\begin{tabular}{l|l|ccccccccccccccccc|c}\hline
    Method & Prompt & \rotatebox[origin=c]{70}{ImageNet} & \rotatebox[origin=c]{70}{ImageNet-C} & \rotatebox[origin=c]{70}{ImageNet-A} & \rotatebox[origin=c]{70}{ImageNet-V2} & \rotatebox[origin=c]{70}{ImageNet-R} & \rotatebox[origin=c]{70}{ImageNet-S} & \rotatebox[origin=c]{70}{ImageNet-D109} & \rotatebox[origin=c]{70}{Flower102} & \rotatebox[origin=c]{70}{DTD} & \rotatebox[origin=c]{70}{Pets} & \rotatebox[origin=c]{70}{Cars} & \rotatebox[origin=c]{70}{UCF101} & \rotatebox[origin=c]{70}{Caltech101} & \rotatebox[origin=c]{70}{Food101} & \rotatebox[origin=c]{70}{SUN397} & \rotatebox[origin=c]{70}{Aircraft} & \rotatebox[origin=c]{70}{EuroSAT} & Avg. \\
    \hline
Source & Single & 20.8 & 45.2 & 24.2 & 27.9 & 8.0 & 32.6 & 20.1 & 22.5 & 40.4 & 6.6 & 9.9 & 24.1 & 2.4 & 11.2 & 25.5 & 67.1 & 44.7 & 25.5\\
Source & Ensemble & 20.2 & 45.0 & 24.0 & 27.1 & 7.3 & 31.8 & 19.3 & 21.9 & 36.6 & 8.4 & 10.0 & 23.9 & 3.0 & 10.8 & 25.4 & 67.7 & 32.6 & 24.4\\
Source & CuPL & 20.5 & 45.1 & 23.8 & 27.5 & 8.1 & 32.6 & 19.5 & - & - & - & - & - & - & - & - & - & - & -\\
Source & All Prompts & 19.9 & 44.5 & 23.1 & 26.7 & 7.1 & 31.9 & 19.2 & - & - & - & - & - & - & - & - & - & - & -\\
\hline
VTE & Ensemble & 19.8 & 47.2 & 14.5 & 25.8 & 6.2 & 31.4 & 17.3 & 21.1 & 35.2 & 8.9 & 10.7 & 23.3 & 2.5 & 11.3 & 25.9 & 65.1 & 39.8 & 23.9\\
\hline
TENT & Ensemble & 20.8 & 42.0 & 23.9 & 27.1 & 6.7 & 32.2 & 18.3 & 21.9 & 36.8 & 8.3 & 9.8 & 23.4 & 3.0 & 10.7 & 25.5 & 67.5 & 31.3 & 24.1\\
ETA & Ensemble & 21.3 & 41.8 & 24.4 & 27.4 & 6.5 & 32.2 & 17.9 & 22.1 & 36.6 & 8.3 & 9.4 & 23.3 & 3.0 & 10.7 & 25.7 & 66.8 & 32.6 & 24.1\\
SAR & Ensemble & 20.7 & 42.2 & 23.7 & 27.1 & 6.9 & 32.1 & 18.4 & 21.8 & 36.6 & 8.5 & 9.8 & 23.3 & 3.0 & 10.6 & 25.5 & 67.5 & 30.8 & 24.0\\
DeYO & Ensemble & 21.7 & 44.6 & 23.4 & 27.3 & 6.6 & 32.7 & 19.0 & 22.2 & 37.1 & 8.0 & 9.3 & 22.3 & 3.2 & 10.9 & 26.4 & 68.0 & 40.2 & 24.9\\
CMF & Ensemble & 21.0 & 39.1 & 24.1 & 27.6 & 6.5 & 32.2 & 17.5 & 23.4 & 38.4 & 8.0 & 9.2 & 22.1 & 2.8 & 10.7 & 25.5 & 67.8 & 33.0 & 24.1\\
ROID & Ensemble & 21.0 & 38.7 & 24.1 & 27.3 & 6.4 & 32.3 & 17.8 & 23.5 & 38.5 & 7.8 & 9.1 & 22.3 & 2.7 & 10.6 & 25.7 & 67.8 & 31.0 & 23.9\\
    \hline
\end{tabular}}
\label{tab:detailed_eva02_l_14}
\end{table*}
\begin{table*}[t]

\centering
\caption{Online classification error rate~(\%) for CLIP with a ViT-H-14 backbone. The model comprises 986.11 million parameters and requires 381.68 billion FLOPS.}
\vskip -0.1in
\scalebox{0.75}{
\tabcolsep4pt
\begin{tabular}{l|l|ccccccccccccccccc|c}\hline
    Method & Prompt & \rotatebox[origin=c]{70}{ImageNet} & \rotatebox[origin=c]{70}{ImageNet-C} & \rotatebox[origin=c]{70}{ImageNet-A} & \rotatebox[origin=c]{70}{ImageNet-V2} & \rotatebox[origin=c]{70}{ImageNet-R} & \rotatebox[origin=c]{70}{ImageNet-S} & \rotatebox[origin=c]{70}{ImageNet-D109} & \rotatebox[origin=c]{70}{Flower102} & \rotatebox[origin=c]{70}{DTD} & \rotatebox[origin=c]{70}{Pets} & \rotatebox[origin=c]{70}{Cars} & \rotatebox[origin=c]{70}{UCF101} & \rotatebox[origin=c]{70}{Caltech101} & \rotatebox[origin=c]{70}{Food101} & \rotatebox[origin=c]{70}{SUN397} & \rotatebox[origin=c]{70}{Aircraft} & \rotatebox[origin=c]{70}{EuroSAT} & Avg. \\
    \hline
Source & Single & 23.2 & 61.2 & 41.2 & 29.8 & 12.2 & 34.8 & 20.8 & 20.1 & 36.4 & 8.1 & 7.0 & 22.7 & 2.8 & 11.7 & 25.0 & 59.4 & 42.0 & 27.0\\ 
Source & Ensemble & 22.1 & 60.3 & 40.6 & 29.1 & 10.7 & 33.4 & 19.2 & 19.6 & 32.7 & 8.3 & 6.7 & 22.2 & 3.3 & 11.5 & 24.9 & 58.0 & 32.9 & 25.6\\ 
Source & CuPL & 22.6 & 60.8 & 39.8 & 29.6 & 14.7 & 34.7 & 20.1 & - & - & - & - & - & - & - & - & - & - & -\\ 
Source & All Prompts & 21.6 & 60.1 & 39.8 & 28.4 & 11.1 & 33.5 & 19.2 & - & - & - & - & - & - & - & - & - & - & -\\ 
\hline
VTE & Ensemble & 22.2 & 62.0 & 30.5 & 29.0 & 10.4 & 34.7 & 18.4 & 18.9 & 33.2 & 8.9 & 7.3 & 23.8 & 3.1 & 13.4 & 26.9 & 57.8 & 46.6 & 26.3\\ 
\hline
TENT & Ensemble & 22.0 & 59.7 & 40.6 & 29.1 & 10.6 & 33.5 & 19.2 & 19.6 & 32.7 & 8.3 & 6.7 & 22.2 & 3.3 & 11.4 & 24.8 & 58.1 & 32.4 & 25.5\\ 
ETA & Ensemble & 21.9 & 54.7 & 43.3 & 29.0 & 10.6 & 33.1 & 19.1 & 19.6 & 32.6 & 8.3 & 6.7 & 22.2 & 3.3 & 11.4 & 24.7 & 58.1 & 33.0 & 25.4\\ 
SAR & Ensemble & 22.1 & 56.6 & 40.6 & 29.0 & 10.7 & 33.2 & 19.2 & 19.6 & 32.6 & 8.3 & 6.7 & 22.3 & 3.3 & 11.5 & 24.8 & 57.8 & 32.6 & 25.3\\ 
DeYO & Ensemble & 22.1 & 54.8 & 40.2 & 28.9 & 10.5 & 33.0 & 18.8 & 19.8 & 32.5 & 8.2 & 6.7 & 22.2 & 3.3 & 11.4 & 24.6 & 57.7 & 31.4 & 25.1\\ 
CMF & Ensemble & 21.9 & 51.8 & 40.0 & 29.0 & 10.3 & 32.6 & 18.5 & 19.7 & 32.8 & 8.3 & 6.7 & 22.3 & 3.2 & 11.3 & 24.6 & 57.7 & 28.1 & 24.6\\ 
ROID & Ensemble & 22.0 & 53.3 & 40.4 & 29.0 & 10.6 & 33.2 & 19.0 & 19.9 & 33.0 & 8.4 & 6.7 & 22.4 & 3.3 & 11.5 & 24.7 & 57.5 & 27.9 & 24.9\\
    \hline
\end{tabular}}
\label{tab:detailed_vit_h_14}
\end{table*}
