# Supplementary material for: A Lost Opportunity for Vision-Language Models: A Comparative Study of Online Test-Time Adaptation for Vision-Language Models
Source: arXiv:2405.14977 source file (2024-09-09)
Supplement: Supplementary file 2 [file eva02-b-16_detailed.tex]

\begin{table*}[t]

\centering
\caption{Online classification error rate~(\%) for CLIP with a EVA02-B-16 backbone. The model comprises 149.69 million parameters and requires 41.09 billion FLOPS.}
\vskip -0.1in
\scalebox{0.75}{
\tabcolsep4pt
\begin{tabular}{l|l|ccccccccccccccccc|c}\hline
    Method & Prompt & \rotatebox[origin=c]{70}{ImageNet} & \rotatebox[origin=c]{70}{ImageNet-C} & \rotatebox[origin=c]{70}{ImageNet-A} & \rotatebox[origin=c]{70}{ImageNet-V2} & \rotatebox[origin=c]{70}{ImageNet-R} & \rotatebox[origin=c]{70}{ImageNet-S} & \rotatebox[origin=c]{70}{ImageNet-D109} & \rotatebox[origin=c]{70}{Flower102} & \rotatebox[origin=c]{70}{DTD} & \rotatebox[origin=c]{70}{Pets} & \rotatebox[origin=c]{70}{Cars} & \rotatebox[origin=c]{70}{UCF101} & \rotatebox[origin=c]{70}{Caltech101} & \rotatebox[origin=c]{70}{Food101} & \rotatebox[origin=c]{70}{SUN397} & \rotatebox[origin=c]{70}{Aircraft} & \rotatebox[origin=c]{70}{EuroSAT} & Avg. \\
    \hline
Source & Single & 25.5 & 64.5 & 46.5 & 33.3 & 18.9 & 42.9 & 26.1 & 24.5 & 50.1 & 10.0 & 20.9 & 31.7 & 2.8 & 15.6 & 29.1 & 77.3 & 45.1 & 33.2\\
Source & Ensemble & 25.3 & 63.8 & 46.1 & 33.0 & 17.6 & 42.3 & 25.0 & 25.1 & 47.7 & 10.2 & 20.9 & 31.2 & 3.6 & 15.1 & 29.1 & 76.7 & 37.8 & 32.4\\
Source & CuPL & 24.8 & 63.9 & 45.8 & 32.5 & 19.3 & 42.7 & 25.2 & - & - & - & - & - & - & - & - & - & - & -\\
Source & All Prompts & 24.6 & 63.5 & 45.4 & 32.2 & 17.5 & 42.1 & 24.8 & - & - & - & - & - & - & - & - & - & - & -\\
\hline
EnsembleCLIP & Ensemble & 23.6 & 63.2 & 27.9 & 30.6 & 14.4 & 40.7 & 21.9 & 26.6 & 46.1 & 11.3 & 19.4 & 32.0 & 3.6 & 15.9 & 30.0 & 76.4 & 48.8 & 31.3\\
\hline
TENT & Ensemble & 25.3 & 94.6 & 43.7 & 32.8 & 15.7 & 41.6 & 32.3 & 25.2 & 48.2 & 10.1 & 20.1 & 31.0 & 3.5 & 15.0 & 29.5 & 77.4 & 34.4 & 34.1\\
ETA & Ensemble & 25.7 & 55.4 & 43.6 & 32.8 & 15.3 & 41.4 & 22.9 & 25.4 & 47.8 & 10.2 & 20.3 & 30.0 & 3.8 & 14.8 & 29.5 & 77.0 & 37.8 & 31.4\\
SAR & Ensemble & 25.1 & 57.4 & 44.3 & 32.8 & 16.6 & 41.7 & 24.2 & 25.0 & 47.9 & 10.1 & 20.1 & 30.8 & 3.7 & 15.1 & 29.1 & 77.2 & 38.0 & 31.7\\
DeYO & Ensemble & 26.0 & 57.4 & 42.4 & 32.8 & 15.4 & 41.9 & 23.8 & 24.6 & 48.5 & 10.4 & 20.4 & 30.3 & 3.5 & 15.3 & 29.6 & 79.0 & 64.5 & 33.3\\
CMF & Ensemble & 25.9 & 51.5 & 43.8 & 33.1 & 15.2 & 41.8 & 22.6 & 25.9 & 49.5 & 9.3 & 21.4 & 30.1 & 4.0 & 15.0 & 29.5 & 78.7 & 44.6 & 31.9\\
ROID & Ensemble & 25.4 & 50.8 & 43.2 & 32.8 & 15.1 & 41.3 & 22.8 & 25.9 & 49.5 & 9.2 & 21.0 & 29.7 & 4.0 & 15.1 & 29.1 & 78.5 & 42.0 & 31.5\\
    \hline
\end{tabular}}
\label{tab:detailed_eva02_b_16}
\end{table*}
