# Supplementary material for: A Lost Opportunity for Vision-Language Models: A Comparative Study of Online Test-Time Adaptation for Vision-Language Models
Source: arXiv:2405.14977 source file (2024-09-09)
Supplement: Supplementary file 3 [file eva02-l-14_detailed.tex]

\begin{table*}[t]

\centering
\caption{Online classification error rate~(\%) for CLIP with a EVA02-L-14 backbone. The model comprises 427.76 million parameters and requires 175.3 billion FLOPS.}
\vskip -0.1in
\scalebox{0.75}{
\tabcolsep4pt
\begin{tabular}{l|l|ccccccccccccccccc|c}\hline
    Method & Prompt & \rotatebox[origin=c]{70}{ImageNet} & \rotatebox[origin=c]{70}{ImageNet-C} & \rotatebox[origin=c]{70}{ImageNet-A} & \rotatebox[origin=c]{70}{ImageNet-V2} & \rotatebox[origin=c]{70}{ImageNet-R} & \rotatebox[origin=c]{70}{ImageNet-S} & \rotatebox[origin=c]{70}{ImageNet-D109} & \rotatebox[origin=c]{70}{Flower102} & \rotatebox[origin=c]{70}{DTD} & \rotatebox[origin=c]{70}{Pets} & \rotatebox[origin=c]{70}{Cars} & \rotatebox[origin=c]{70}{UCF101} & \rotatebox[origin=c]{70}{Caltech101} & \rotatebox[origin=c]{70}{Food101} & \rotatebox[origin=c]{70}{SUN397} & \rotatebox[origin=c]{70}{Aircraft} & \rotatebox[origin=c]{70}{EuroSAT} & Avg. \\
    \hline
Source & Single & 20.8 & 45.2 & 24.2 & 27.9 & 8.0 & 32.6 & 20.1 & 22.5 & 40.4 & 6.6 & 9.9 & 24.1 & 2.4 & 11.2 & 25.5 & 67.1 & 44.7 & 25.5\\
Source & Ensemble & 20.2 & 45.0 & 24.0 & 27.1 & 7.3 & 31.8 & 19.3 & 21.9 & 36.6 & 8.4 & 10.0 & 23.9 & 3.0 & 10.8 & 25.4 & 67.7 & 32.6 & 24.4\\
Source & CuPL & 20.5 & 45.1 & 23.8 & 27.5 & 8.1 & 32.6 & 19.5 & - & - & - & - & - & - & - & - & - & - & -\\
Source & All Prompts & 19.9 & 44.5 & 23.1 & 26.7 & 7.1 & 31.9 & 19.2 & - & - & - & - & - & - & - & - & - & - & -\\
\hline
VTE & Ensemble & 19.8 & 47.2 & 14.5 & 25.8 & 6.2 & 31.4 & 17.3 & 21.1 & 35.2 & 8.9 & 10.7 & 23.3 & 2.5 & 11.3 & 25.9 & 65.1 & 39.8 & 23.9\\
\hline
TENT & Ensemble & 20.8 & 42.0 & 23.9 & 27.1 & 6.7 & 32.2 & 18.3 & 21.9 & 36.8 & 8.3 & 9.8 & 23.4 & 3.0 & 10.7 & 25.5 & 67.5 & 31.3 & 24.1\\
ETA & Ensemble & 21.3 & 41.8 & 24.4 & 27.4 & 6.5 & 32.2 & 17.9 & 22.1 & 36.6 & 8.3 & 9.4 & 23.3 & 3.0 & 10.7 & 25.7 & 66.8 & 32.6 & 24.1\\
SAR & Ensemble & 20.7 & 42.2 & 23.7 & 27.1 & 6.9 & 32.1 & 18.4 & 21.8 & 36.6 & 8.5 & 9.8 & 23.3 & 3.0 & 10.6 & 25.5 & 67.5 & 30.8 & 24.0\\
DeYO & Ensemble & 21.7 & 44.6 & 23.4 & 27.3 & 6.6 & 32.7 & 19.0 & 22.2 & 37.1 & 8.0 & 9.3 & 22.3 & 3.2 & 10.9 & 26.4 & 68.0 & 40.2 & 24.9\\
CMF & Ensemble & 21.0 & 39.1 & 24.1 & 27.6 & 6.5 & 32.2 & 17.5 & 23.4 & 38.4 & 8.0 & 9.2 & 22.1 & 2.8 & 10.7 & 25.5 & 67.8 & 33.0 & 24.1\\
ROID & Ensemble & 21.0 & 38.7 & 24.1 & 27.3 & 6.4 & 32.3 & 17.8 & 23.5 & 38.5 & 7.8 & 9.1 & 22.3 & 2.7 & 10.6 & 25.7 & 67.8 & 31.0 & 23.9\\
    \hline
\end{tabular}}
\label{tab:detailed_eva02_l_14}
\end{table*}
