# Supplementary material for: A Lost Opportunity for Vision-Language Models: A Comparative Study of Online Test-Time Adaptation for Vision-Language Models
Source: arXiv:2405.14977 source file (2024-09-09)
Supplement: Supplementary file 4 [file rn50_detailed.tex]

\begin{table*}[t]

\centering
\caption{Online classification error rate~(\%) for CLIP with a RN50 backbone pretrained by OpenAI. The model comprises 102.01 million parameters and requires 18.18 billion FLOPS.}
\vskip -0.1in
\scalebox{0.75}{
\tabcolsep4pt
\begin{tabular}{l|l|ccccccccccccccccc|c}\hline
    Method & Prompt & \rotatebox[origin=c]{70}{ImageNet} & \rotatebox[origin=c]{70}{ImageNet-C} & \rotatebox[origin=c]{70}{ImageNet-A} & \rotatebox[origin=c]{70}{ImageNet-V2} & \rotatebox[origin=c]{70}{ImageNet-R} & \rotatebox[origin=c]{70}{ImageNet-S} & \rotatebox[origin=c]{70}{ImageNet-D109} & \rotatebox[origin=c]{70}{Flower102} & \rotatebox[origin=c]{70}{DTD} & \rotatebox[origin=c]{70}{Pets} & \rotatebox[origin=c]{70}{Cars} & \rotatebox[origin=c]{70}{UCF101} & \rotatebox[origin=c]{70}{Caltech101} & \rotatebox[origin=c]{70}{Food101} & \rotatebox[origin=c]{70}{SUN397} & \rotatebox[origin=c]{70}{Aircraft} & \rotatebox[origin=c]{70}{EuroSAT} & Avg. \\
    \hline
Source & Single & 41.8 & 89.0 & 78.3 & 48.5 & 44.1 & 66.7 & 41.2 & 39.0 & 60.1 & 16.4 & 44.4 & 41.7 & 14.1 & 26.2 & 41.4 & 84.4 & 75.8 & 50.2 \\ 
Source & Ensemble & 40.2 & 88.3 & 77.3 & 47.2 & 39.4 & 64.6 & 38.7 & 38.7 & 58.3 & 16.7 & 44.0 & 40.6 & 13.8 & 24.3 & 39.8 & 83.0 & 61.8 & 48.0 \\ 
Source & CuPL & 38.5 & 87.7 & 76.2 & 45.4 & 40.0 & 64.3 & 38.6 & - & - & - & - & - & - & - & - & - & - & -\ \\ 
Source & All Prompts & 38.7 & 87.8 & 76.2 & 45.9 & 38.9 & 63.7 & 38.2 & - & - & - & - & - & - & - & - & - & - & -\ \\ 
\hline
TPT & a photo of a & 39.2 & 88.6 & 73.7 & 45.5 & 41.1 & 64.8 & 38.4 & 37.8 & 59.0 & 15.2 & 41.4 & 40.3 & 13.1 & 25.1 & 38.7 & 82.8 & 72.0 & 48.0 \\ 
VTE & Ensemble & 38.6 & 88.5 & 66.5 & 44.5 & 37.8 & 63.0 & 36.1 & 41.6 & 59.4 & 17.3 & 41.3 & 41.0 & 13.5 & 26.4 & 39.1 & 81.1 & 72.7 & 47.5 \\ 
\hline
TENT & Ensemble & 53.3 & 97.8 & 89.8 & 59.8 & 56.6 & 82.1 & 50.7 & 88.6 & 78.2 & 52.0 & 91.3 & 61.2 & 35.9 & 90.2 & 60.1 & 95.8 & 87.8 & 72.4 \\ 
ETA & Ensemble & 50.2 & 99.8 & 89.5 & 58.8 & 53.4 & 78.9 & 49.5 & 88.6 & 78.3 & 52.2 & 91.0 & 61.5 & 36.3 & 85.2 & 58.4 & 95.8 & 86.9 & 71.4 \\ 
SAR & Ensemble & 53.7 & 96.2 & 89.8 & 59.9 & 57.4 & 81.8 & 51.0 & 88.4 & 78.2 & 52.0 & 91.0 & 61.1 & 36.5 & 88.1 & 60.2 & 95.7 & 86.9 & 72.2 \\ 
DeYO & Ensemble & 50.1 & 99.8 & 89.4 & 58.3 & 52.6 & 79.9 & 48.2 & 88.9 & 77.9 & 51.2 & 90.7 & 60.5 & 34.7 & 89.5 & 57.8 & 96.3 & 89.1 & 71.5 \\ 
CMF & Ensemble & 48.0 & 93.3 & 88.4 & 57.2 & 47.0 & 75.2 & 44.6 & 88.8 & 78.2 & 44.6 & 90.2 & 57.0 & 33.5 & 80.1 & 54.1 & 95.7 & 91.1 & 68.6 \\ 
ROID & Ensemble & 50.2 & 91.7 & 89.0 & 57.2 & 50.2 & 77.8 & 47.1 & 89.0 & 77.9 & 44.8 & 90.4 & 57.4 & 33.1 & 83.9 & 55.9 & 95.9 & 90.6 & 69.5 \\
    \hline
\end{tabular}}
\label{tab:detailed_rn50}
\end{table*}
