# Supplementary material for: A Lost Opportunity for Vision-Language Models: A Comparative Study of Online Test-Time Adaptation for Vision-Language Models
Source: arXiv:2405.14977 source file (2024-09-09)
Supplement: Supplementary file 5 [file vit-b-16_detailed.tex]

\begin{table*}[t]

\centering
\caption{Online classification error rate~(\%) for CLIP with a ViT-B-16 backbone pretrained by OpenAI. The model comprises 149.62 million parameters and requires 41.09 billion FLOPS.}
\vskip -0.1in
\scalebox{0.75}{
\tabcolsep4pt
\begin{tabular}{l|l|ccccccccccccccccc|c}\hline
    Method & Prompt & \rotatebox[origin=c]{70}{ImageNet} & \rotatebox[origin=c]{70}{ImageNet-C} & \rotatebox[origin=c]{70}{ImageNet-A} & \rotatebox[origin=c]{70}{ImageNet-V2} & \rotatebox[origin=c]{70}{ImageNet-R} & \rotatebox[origin=c]{70}{ImageNet-S} & \rotatebox[origin=c]{70}{ImageNet-D109} & \rotatebox[origin=c]{70}{Flower102} & \rotatebox[origin=c]{70}{DTD} & \rotatebox[origin=c]{70}{Pets} & \rotatebox[origin=c]{70}{Cars} & \rotatebox[origin=c]{70}{UCF101} & \rotatebox[origin=c]{70}{Caltech101} & \rotatebox[origin=c]{70}{Food101} & \rotatebox[origin=c]{70}{SUN397} & \rotatebox[origin=c]{70}{Aircraft} & \rotatebox[origin=c]{70}{EuroSAT} & Avg. \\
    \hline
Source & Single & 33.3 & 75.5 & 52.3 & 39.2 & 26.0 & 53.9 & 29.5 & 32.6 & 55.4 & 11.8 & 34.8 & 34.9 & 7.1 & 16.2 & 37.4 & 76.2 & 58.5 & 39.7\\ 
Source & Ensemble & 31.7 & 73.8 & 49.9 & 38.1 & 22.5 & 51.7 & 27.5 & 34.2 & 54.6 & 11.8 & 33.6 & 32.6 & 7.0 & 15.5 & 34.6 & 76.5 & 51.8 & 38.1\\ 
Source & CuPL & 30.4 & 73.3 & 49.3 & 36.7 & 22.9 & 51.0 & 28.0 & - & - & - & - & - & - & - & - & - & - & -\\ 
Source & All Prompts & 30.3 & 73.0 & 49.0 & 36.9 & 22.0 & 50.6 & 27.2 & - & - & - & - & - & - & - & - & - & - & -\\ 
\hline
TPT & a photo of a & 31.0 & 75.1 & 45.7 & 36.5 & 23.0 & 52.2 & 26.8 & 30.9 & 52.7 & 12.8 & 34.0 & 32.5 & 6.3 & 15.2 & 34.6 & 76.7 & 57.2 & 37.8\\ 
VTE & Ensemble & 29.6 & 74.4 & 37.3 & 34.9 & 19.6 & 49.8 & 24.6 & 34.5 & 52.7 & 13.0 & 31.0 & 33.0 & 6.7 & 16.6 & 33.5 & 75.9 & 52.4 & 36.4\\ 
\hline
TENT & Ensemble & 31.6 & 75.4 & 49.6 & 38.1 & 21.6 & 51.6 & 27.2 & 34.2 & 54.3 & 11.6 & 33.6 & 32.3 & 6.9 & 15.8 & 34.4 & 76.5 & 43.3 & 37.5\\ 
ETA & Ensemble & 32.1 & 69.1 & 49.3 & 38.3 & 21.7 & 50.9 & 26.9 & 34.0 & 54.4 & 11.3 & 33.5 & 32.1 & 7.0 & 16.0 & 33.9 & 76.2 & 50.7 & 37.5\\ 
SAR & Ensemble & 32.0 & 70.0 & 49.2 & 38.3 & 21.8 & 51.5 & 27.0 & 33.9 & 54.4 & 11.5 & 34.1 & 32.5 & 7.0 & 15.7 & 34.8 & 76.4 & 44.7 & 37.3\\ 
DeYO & Ensemble & 32.4 & 71.3 & 48.9 & 38.4 & 21.7 & 51.5 & 27.0 & 34.2 & 54.3 & 11.3 & 34.1 & 32.1 & 7.2 & 16.0 & 35.0 & 76.2 & 50.1 & 37.7\\ 
CMF & Ensemble & 31.9 & 66.1 & 49.6 & 38.3 & 20.9 & 50.4 & 25.7 & 33.8 & 54.4 & 11.5 & 33.8 & 32.0 & 6.9 & 15.7 & 33.6 & 76.3 & 36.5 & 36.3\\ 
ROID & Ensemble & 31.7 & 65.7 & 49.3 & 38.2 & 21.1 & 50.9 & 26.3 & 33.6 & 54.2 & 11.4 & 33.4 & 31.9 & 6.9 & 15.8 & 33.4 & 76.1 & 36.3 & 36.2 \\
    \hline
\end{tabular}}
\label{tab:detailed_vit_b_16}
\end{table*}
