# Supplementary material for: A Lost Opportunity for Vision-Language Models: A Comparative Study of Online Test-Time Adaptation for Vision-Language Models
Source: arXiv:2405.14977 source file (2024-09-09)
Supplement: Supplementary file 6 [file vit-h-14_detailed.tex]

\begin{table*}[t]

\centering
\caption{Online classification error rate~(\%) for CLIP with a ViT-H-14 backbone. The model comprises 986.11 million parameters and requires 381.68 billion FLOPS.}
\vskip -0.1in
\scalebox{0.75}{
\tabcolsep4pt
\begin{tabular}{l|l|ccccccccccccccccc|c}\hline
    Method & Prompt & \rotatebox[origin=c]{70}{ImageNet} & \rotatebox[origin=c]{70}{ImageNet-C} & \rotatebox[origin=c]{70}{ImageNet-A} & \rotatebox[origin=c]{70}{ImageNet-V2} & \rotatebox[origin=c]{70}{ImageNet-R} & \rotatebox[origin=c]{70}{ImageNet-S} & \rotatebox[origin=c]{70}{ImageNet-D109} & \rotatebox[origin=c]{70}{Flower102} & \rotatebox[origin=c]{70}{DTD} & \rotatebox[origin=c]{70}{Pets} & \rotatebox[origin=c]{70}{Cars} & \rotatebox[origin=c]{70}{UCF101} & \rotatebox[origin=c]{70}{Caltech101} & \rotatebox[origin=c]{70}{Food101} & \rotatebox[origin=c]{70}{SUN397} & \rotatebox[origin=c]{70}{Aircraft} & \rotatebox[origin=c]{70}{EuroSAT} & Avg. \\
    \hline
Source & Single & 23.2 & 61.2 & 41.2 & 29.8 & 12.2 & 34.8 & 20.8 & 20.1 & 36.4 & 8.1 & 7.0 & 22.7 & 2.8 & 11.7 & 25.0 & 59.4 & 42.0 & 27.0\\ 
Source & Ensemble & 22.1 & 60.3 & 40.6 & 29.1 & 10.7 & 33.4 & 19.2 & 19.6 & 32.7 & 8.3 & 6.7 & 22.2 & 3.3 & 11.5 & 24.9 & 58.0 & 32.9 & 25.6\\ 
Source & CuPL & 22.6 & 60.8 & 39.8 & 29.6 & 14.7 & 34.7 & 20.1 & - & - & - & - & - & - & - & - & - & - & -\\ 
Source & All Prompts & 21.6 & 60.1 & 39.8 & 28.4 & 11.1 & 33.5 & 19.2 & - & - & - & - & - & - & - & - & - & - & -\\ 
\hline
VTE & Ensemble & 22.2 & 62.0 & 30.5 & 29.0 & 10.4 & 34.7 & 18.4 & 18.9 & 33.2 & 8.9 & 7.3 & 23.8 & 3.1 & 13.4 & 26.9 & 57.8 & 46.6 & 26.3\\ 
\hline
TENT & Ensemble & 22.0 & 59.7 & 40.6 & 29.1 & 10.6 & 33.5 & 19.2 & 19.6 & 32.7 & 8.3 & 6.7 & 22.2 & 3.3 & 11.4 & 24.8 & 58.1 & 32.4 & 25.5\\ 
ETA & Ensemble & 21.9 & 54.7 & 43.3 & 29.0 & 10.6 & 33.1 & 19.1 & 19.6 & 32.6 & 8.3 & 6.7 & 22.2 & 3.3 & 11.4 & 24.7 & 58.1 & 33.0 & 25.4\\ 
SAR & Ensemble & 22.1 & 56.6 & 40.6 & 29.0 & 10.7 & 33.2 & 19.2 & 19.6 & 32.6 & 8.3 & 6.7 & 22.3 & 3.3 & 11.5 & 24.8 & 57.8 & 32.6 & 25.3\\ 
DeYO & Ensemble & 22.1 & 54.8 & 40.2 & 28.9 & 10.5 & 33.0 & 18.8 & 19.8 & 32.5 & 8.2 & 6.7 & 22.2 & 3.3 & 11.4 & 24.6 & 57.7 & 31.4 & 25.1\\ 
CMF & Ensemble & 21.9 & 51.8 & 40.0 & 29.0 & 10.3 & 32.6 & 18.5 & 19.7 & 32.8 & 8.3 & 6.7 & 22.3 & 3.2 & 11.3 & 24.6 & 57.7 & 28.1 & 24.6\\ 
ROID & Ensemble & 22.0 & 53.3 & 40.4 & 29.0 & 10.6 & 33.2 & 19.0 & 19.9 & 33.0 & 8.4 & 6.7 & 22.4 & 3.3 & 11.5 & 24.7 & 57.5 & 27.9 & 24.9\\
    \hline
\end{tabular}}
\label{tab:detailed_vit_h_14}
\end{table*}
