# Supplementary material for: A Lost Opportunity for Vision-Language Models: A Comparative Study of Online Test-Time Adaptation for Vision-Language Models
Source: arXiv:2405.14977 source file (2024-09-09)
Supplement: Supplementary file 7 [file vit-l-14_detailed.tex]

\begin{table*}[t]

\centering
\caption{Online classification error rate~(\%) for CLIP with a ViT-L-14 backbone pretrained by OpenAI. The model comprises 427.62 million parameters and requires 175.33 billion FLOPS.}
\vskip -0.1in
\scalebox{0.75}{
\tabcolsep4pt
\begin{tabular}{l|l|ccccccccccccccccc|c}\hline
    Method & Prompt & \rotatebox[origin=c]{70}{ImageNet} & \rotatebox[origin=c]{70}{ImageNet-C} & \rotatebox[origin=c]{70}{ImageNet-A} & \rotatebox[origin=c]{70}{ImageNet-V2} & \rotatebox[origin=c]{70}{ImageNet-R} & \rotatebox[origin=c]{70}{ImageNet-S} & \rotatebox[origin=c]{70}{ImageNet-D109} & \rotatebox[origin=c]{70}{Flower102} & \rotatebox[origin=c]{70}{DTD} & \rotatebox[origin=c]{70}{Pets} & \rotatebox[origin=c]{70}{Cars} & \rotatebox[origin=c]{70}{UCF101} & \rotatebox[origin=c]{70}{Caltech101} & \rotatebox[origin=c]{70}{Food101} & \rotatebox[origin=c]{70}{SUN397} & \rotatebox[origin=c]{70}{Aircraft} & \rotatebox[origin=c]{70}{EuroSAT} & Avg. \\
    \hline
Source & Single & 26.5 & 60.5 & 31.3 & 32.1 & 14.6 & 42.1 & 24.2 & 24.1 & 47.4 & 6.8 & 23.2 & 27.3 & 5.2 & 11.4 & 32.5 & 69.7 & 44.7 & 30.8\\ 
Source & Ensemble & 24.5 & 58.6 & 29.3 & 30.1 & 12.2 & 40.4 & 22.4 & 24.4 & 43.3 & 7.0 & 22.1 & 25.0 & 5.5 & 10.8 & 30.9 & 68.1 & 39.3 & 29.1\\ 
Source & CuPL & 23.4 & 57.7 & 28.2 & 29.2 & 12.3 & 40.0 & 22.5 & - & - & - & - & - & - & - & - & - & - & -\\ 
Source & All Prompts & 23.5 & 57.5 & 28.2 & 29.0 & 11.8 & 39.7 & 22.1 & - & - & - & - & - & - & - & - & - & - & -\\ 
\hline
TPT & a photo of a & 24.5 & 59.0 & 25.2 & 29.9 & 12.1 & 40.2 & 22.0 & 23.5 & 46.1 & 6.4 & 22.3 & 25.5 & 4.4 & 10.9 & 29.8 & 68.7 & 48.0 & 29.3\\ 
VTE & Ensemble & 23.0 & 59.5 & 20.4 & 28.4 & 10.3 & 38.9 & 20.5 & 26.2 & 41.9 & 7.1 & 21.6 & 24.6 & 4.2 & 11.7 & 29.3 & 66.1 & 46.4 & 28.2\\ 
\hline
TENT & Ensemble & 24.6 & 56.1 & 29.3 & 30.3 & 12.1 & 40.1 & 22.1 & 24.4 & 43.2 & 6.9 & 22.2 & 24.9 & 5.6 & 10.8 & 30.8 & 68.0 & 36.5 & 28.7\\ 
ETA & Ensemble & 24.6 & 53.8 & 28.9 & 30.4 & 11.9 & 39.6 & 21.7 & 24.3 & 43.1 & 7.0 & 21.7 & 24.7 & 5.6 & 10.8 & 30.5 & 67.8 & 39.3 & 28.6\\ 
SAR & Ensemble & 24.6 & 54.9 & 28.9 & 30.3 & 11.8 & 39.8 & 21.9 & 24.3 & 43.2 & 6.9 & 22.1 & 24.9 & 5.6 & 10.7 & 30.4 & 68.0 & 36.2 & 28.5\\ 
DeYO & Ensemble & 24.6 & 54.3 & 28.6 & 30.5 & 11.6 & 39.6 & 21.3 & 24.3 & 43.1 & 6.8 & 21.8 & 24.9 & 5.7 & 10.9 & 30.7 & 67.9 & 38.1 & 28.5\\ 
CMF & Ensemble & 24.2 & 50.6 & 28.2 & 30.0 & 11.1 & 38.6 & 20.4 & 24.1 & 43.0 & 6.6 & 21.9 & 24.7 & 5.6 & 10.7 & 30.1 & 67.4 & 32.2 & 27.6\\ 
ROID & Ensemble & 24.3 & 51.4 & 28.4 & 30.0 & 11.6 & 39.3 & 21.5 & 23.9 & 43.3 & 6.6 & 21.8 & 24.7 & 5.6 & 10.7 & 30.1 & 67.6 & 32.3 & 27.8\\
    \hline
\end{tabular}}
\label{tab:detailed_vit_l_14}
\end{table*}
